# Supplementary material for: TeDiO: Temporal Diagonal Optimization for Training-Free Coherent Video Diffusion
Source: arXiv:2605.14136 source file (2026-05-13)
Supplement: Supplementary file 1 [file X_suppl.tex]

\clearpage
\setcounter{page}{1}
\maketitlesupplementary

\section{Block ablations}

To understand which parts of the diffusion transformer contribute most to temporal coherence, we independently apply TeDiO to each DiT block of Wan2.1-1.3B and evaluate temporal metrics on VideoJam-Bench. Table \ref{tab:block} reports the full results.

Overall, Blocks 2–5 and 22–27 exhibit the strongest impact on temporal stability, with substantial improvements in Motion Smoothness, Subject Consistency, and Background Consistency. These blocks correspond to early and mid-level layers of the DiT, which control large-scale motion propagation and cross-frame attention alignment. Optimizing these layers consistently reduces temporal jitter and enhances motion continuity.

Later blocks (e.g., 28–29) produce substantially weaker gains and in some cases degrade Dynamic Degree or visual quality, suggesting that very deep layers specialize more in frame-wise appearance refinement rather than temporal structure, making them less suitable for temporal correction.

Although several early and mid-level DiT blocks improve temporal metrics, we select Block 5 for TeDiO in all main-paper experiments. As shown in Table S3, Block 5 provides the most balanced trade-off across all temporal and perceptual metrics: it achieves high Motion Smoothness ($98.21$), strong Subject and Background Consistency ($94.78$, $96.24$), and maintains competitive Dynamic Degree. While Blocks 2–3 offer slightly higher smoothness, they also suppress motion more aggressively (lower Dynamic Degree), and deeper blocks (e.g., 22–27) yield inconsistent improvements or degrade aesthetic/image quality. Block 5 therefore represents a stable, reliable operating point—early enough to influence global motion propagation, but deep enough to avoid oversmoothing or impacting appearance quality. This makes it the most effective and robust choice for TeDiO across diverse prompts and models.

\begin{table*}[h!]
    \centering
    \caption{Block ablations}
    \begin{tabular}{l|cccccc}
    \toprule
         \begin{tabular}{@{}c@{}}DiT \\ Block \end{tabular}  & \begin{tabular}{@{}c@{}}Motion \\ Smoothness \end{tabular} $\uparrow$ & \begin{tabular}{@{}c@{}}Dynamic \\ Degree \end{tabular} $\uparrow$ & \begin{tabular}{@{}c@{}}Subject \\ Consistency  \end{tabular} $\uparrow$ & \begin{tabular}{@{}c@{}}Background \\ Consistency \end{tabular} $\uparrow$ & \begin{tabular}{@{}c@{}}Aesthetic \\ Quality \end{tabular} $\uparrow$ & \begin{tabular}{@{}c@{}}Imaging \\ Quality \end{tabular} $\uparrow$ \\
         \midrule
         No  & 97.59 & 81.25 & 93.10 & 95.41  & 58.35 & 66.38 \\
         Block 1 & 97.58 & 81.25 & 93.14 & 95.51 & 58.63 & 66.55\\
         Block 2 & 98.63 & 54.69 & 95.02 & 96.44 & 59.89 & 68.97\\
         Block 3 & 98.68 & 53.13 & 95.02 & 96.46 & 60.33 & 68.54\\
         Block 4 & 98.31 & 67.19 & 93.96 & 95.89 & 59.70 & 67.60\\
         Block 5 & 98.21 & 70.31 & 94.78 & 96.24 & 59.22 & 67.84\\
         Block 6 & 98.45 & 43.75 & 94.61 & 96.24 & 59.69 & 67.43\\
         Block 7 & 97.89 & 75.00 & 93.64 & 95.64 & 59.40 & 66.98\\
         Block 8 & 98.31 & 62.50 & 94.22 & 95.79 & 60.66 & 67.90\\
         Block 9 & 97.67 & 80.47 & 92.81 & 95.25 & 59.03 & 66.26\\
         Block 10 & 97.49 & 82.81 & 92.85 & 95.02 & 58.80 & 66.17\\
         Block 11 & 97.91 & 71.88 & 93.53 & 95.45 & 58.83 & 66.50\\
         Block 12 & 97.84 & 75.00 & 93.31 & 95.38 & 59.23 & 67.31\\
         Block 13 & 97.72 & 74.22 & 93.37 & 95.47 & 59.01 & 66.65\\
         Block 14 & 97.74 & 77.34 & 93.11 & 95.28 & 59.38 & 66.67\\
         Block 15 & 97.49 & 81.25 & 93.03 & 95.37 & 58.78 & 66.04\\
         Block 16 & 97.75 & 77.34 & 93.21 & 95.35 & 58.46 & 66.11\\
         Block 17 & 97.51 & 75.78 & 92.97 & 95.24 & 58.60 & 66.34\\
         Block 18 & 97.86 & 74.22 & 93.46 & 95.61 & 58.45 & 67.29\\
         Block 19 & 97.73 & 75.78 & 93.38 & 95.41 & 58.99 & 67.09\\
         Block 20 & 97.66 & 76.56 & 93.40 & 95.45 & 59.60 & 66.80\\
         Block 21 & 97.70 & 77.34 & 93.57 & 95.49 & 58.50 & 67.22\\
         Block 22 & 98.17 & 58.59 & 94.48 & 96.07 & 59.32 & 68.05\\
         Block 23 & 97.82 & 75.78 & 93.75 & 95.44 & 59.27 & 6.14\\
         Block 24 & 97.80 & 69.53 & 93.58 & 95.21 & 59.16 & 67.10\\
         Block 25 & 97.96 & 69.53 & 93.68 & 95.61 & 59.31 & 66.74\\
         Block 26 & 97.82 & 73.44 & 93.51 & 95.57 & 58.80 & 67.52\\
         Block 27 & 98.14 & 60.94 & 94.51 & 96.28 & 60.07 & 67.99\\
         Block 28 & 96.76 & 81.25 & 91.30 & 94.32 & 56.78 & 64.39\\
         Block 29 & 97.02 & 86.72 & 92.04 & 94.44 & 57.93 & 65.71\\
         \bottomrule
    \end{tabular}
    \label{tab:block}
\end{table*}

\section{Supplementary Videos}

To complement our quantitative and qualitative results, we also include supplementary MP4 videos for all models evaluated in the paper. We also provide pptx presentation files with pairs of videos. For each prompt, we generate videos using the same random seed, enabling strict one-to-one visual comparison between:
\begin{itemize}
    \item Wan2.1-1.3B $\rightarrow$ Wan2.1-1.3B + TeDiO
    \item CogVideoX-5B $\rightarrow$ CogVideoX-5B + TeDiO
\end{itemize}

All videos are provided in their native resolution and frame rate. These clips more clearly reveal the improvements TeDiO provides - such as reduced flickering, smoother trajectories, and more consistent motion - that can be difficult to fully appreciate from static frames in the main paper.

Because temporal coherence is inherently a dynamic property, the frame excerpts shown in the paper offer only a partial view of TeDiO’s effects; the accompanying videos allow reviewers to observe the full temporal behavior.
